# Supplementary material for: HOC-Search: Efficient CAD Model and Pose Retrieval from RGB-D Scans
Source: arXiv:2309.06107 source file (2023-09-12)
Supplement: Supplementary file 2 [file supp_unknown_catFigure.tex]

\definecolor{chair_color}{rgb}{0.301, 0.745, 0.933}
\definecolor{cabinet_color}{rgb}{0.494, 0.184, 0.556}
\definecolor{bed_color}{rgb}{0.466, 0.674, 0.188}
\definecolor{sofa_color}{rgb}{0.635, 0.078, 0.184}
\definecolor{table_color}{rgb}{0.000, 0.667, 0.000}
\definecolor{bookshelf_color}{rgb}{0.000, 0.000, 1.000}
\definecolor{lamp_color}{rgb}{1.000, 0.333, 0.500}
\definecolor{display_color}{rgb}{0.333, 0.667, 1.000}

\begin{figure*}
\centering
\scalebox{0.85}{
\begin{tabular}{cccc}
%[trim={left bottom right top}
% \includegraphics[trim={2cm 4cm 4cm 3cm},clip,width=0.25\linewidth]{figures/results_HOC_unknown_cat/scene0549_01/scene_boxes.png} &
%  \includegraphics[trim={2cm 4cm 4cm 3cm},clip,width=0.25\linewidth]{figures/results_HOC_unknown_cat/scene0549_01/exh_search.png} &
%  \includegraphics[trim={2cm 4cm 4cm 3cm},clip,width=0.25\linewidth]{figures/results_HOC_unknown_cat/scene0549_01/hoc_800.png} &
%  \includegraphics[trim={2cm 4cm 4cm 3cm},clip,width=0.25\linewidth]{figures/results_HOC_unknown_cat/scene0549_01/hoc_1200.png} \\

 \includegraphics[trim={7cm 3cm 8cm 4cm},clip,width=0.25\linewidth]{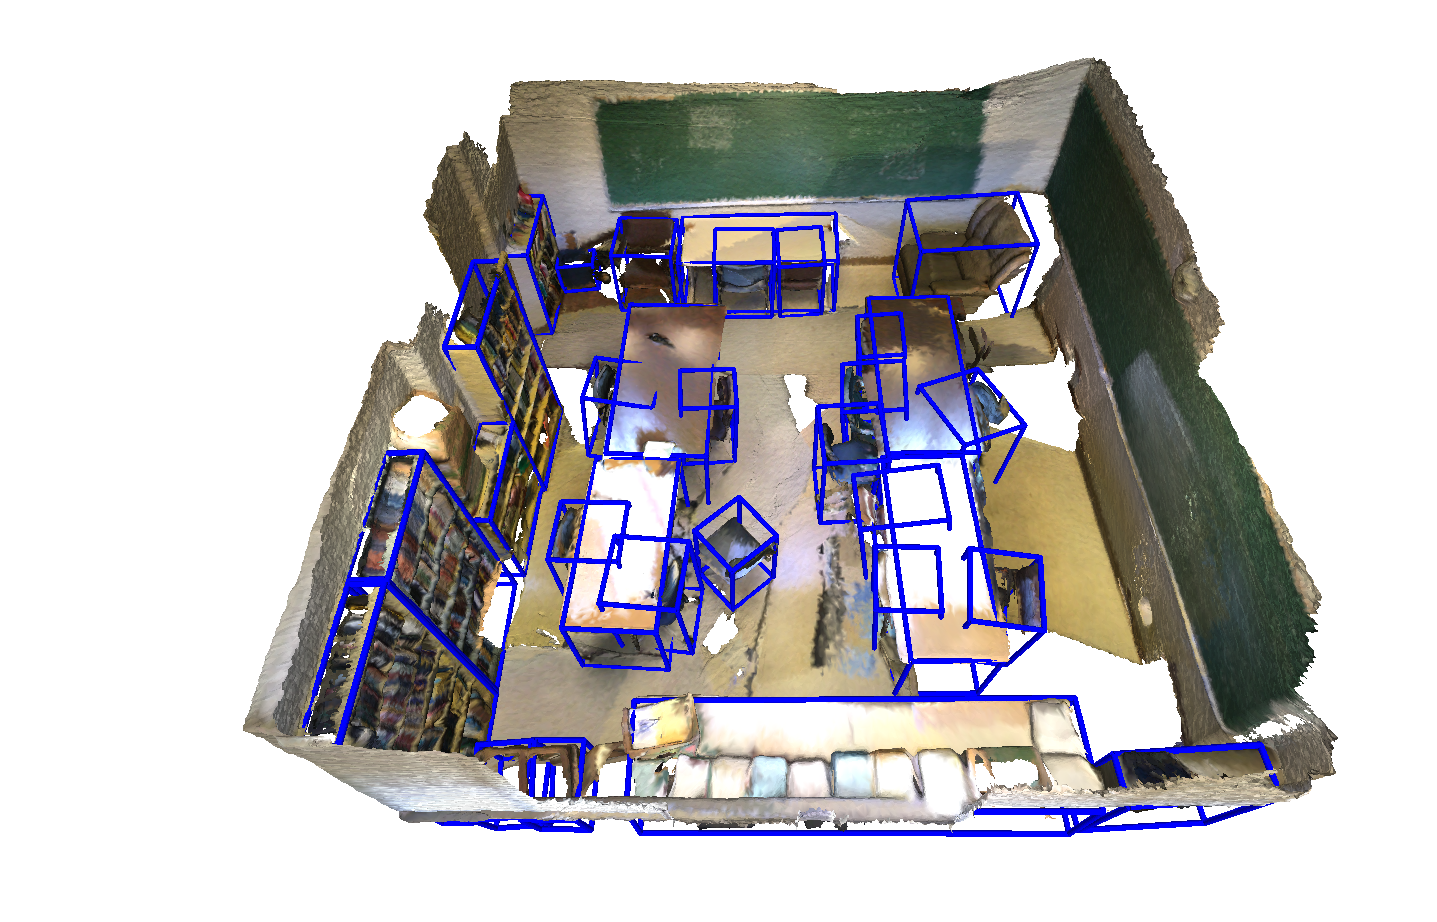} &
  \includegraphics[trim={7cm 3cm 8cm 4cm},clip,width=0.25\linewidth]{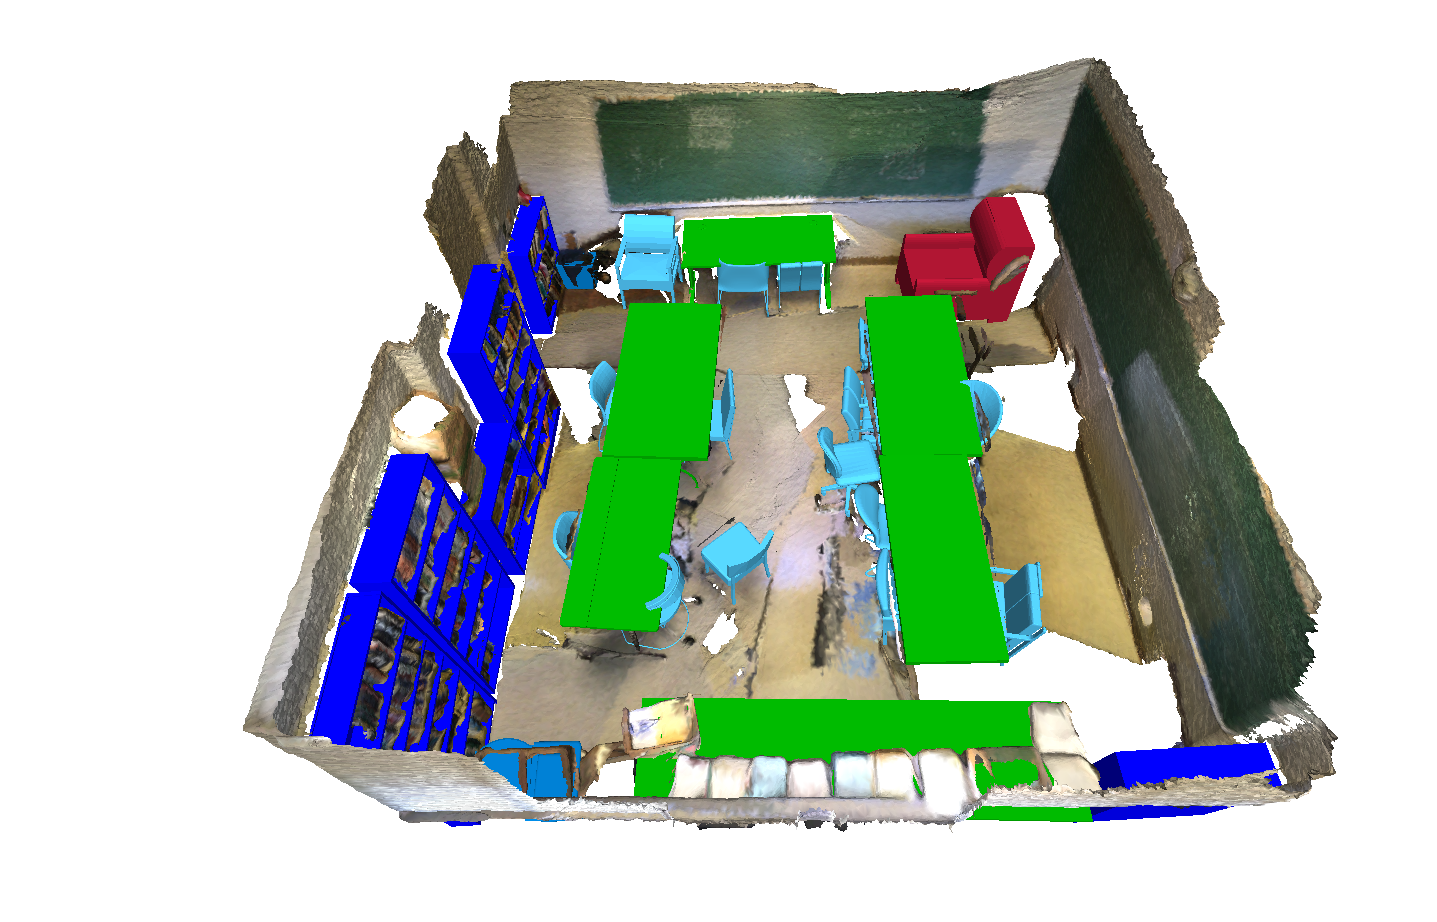} &
  \includegraphics[trim={7cm 3cm 8cm 4cm},clip,width=0.25\linewidth]{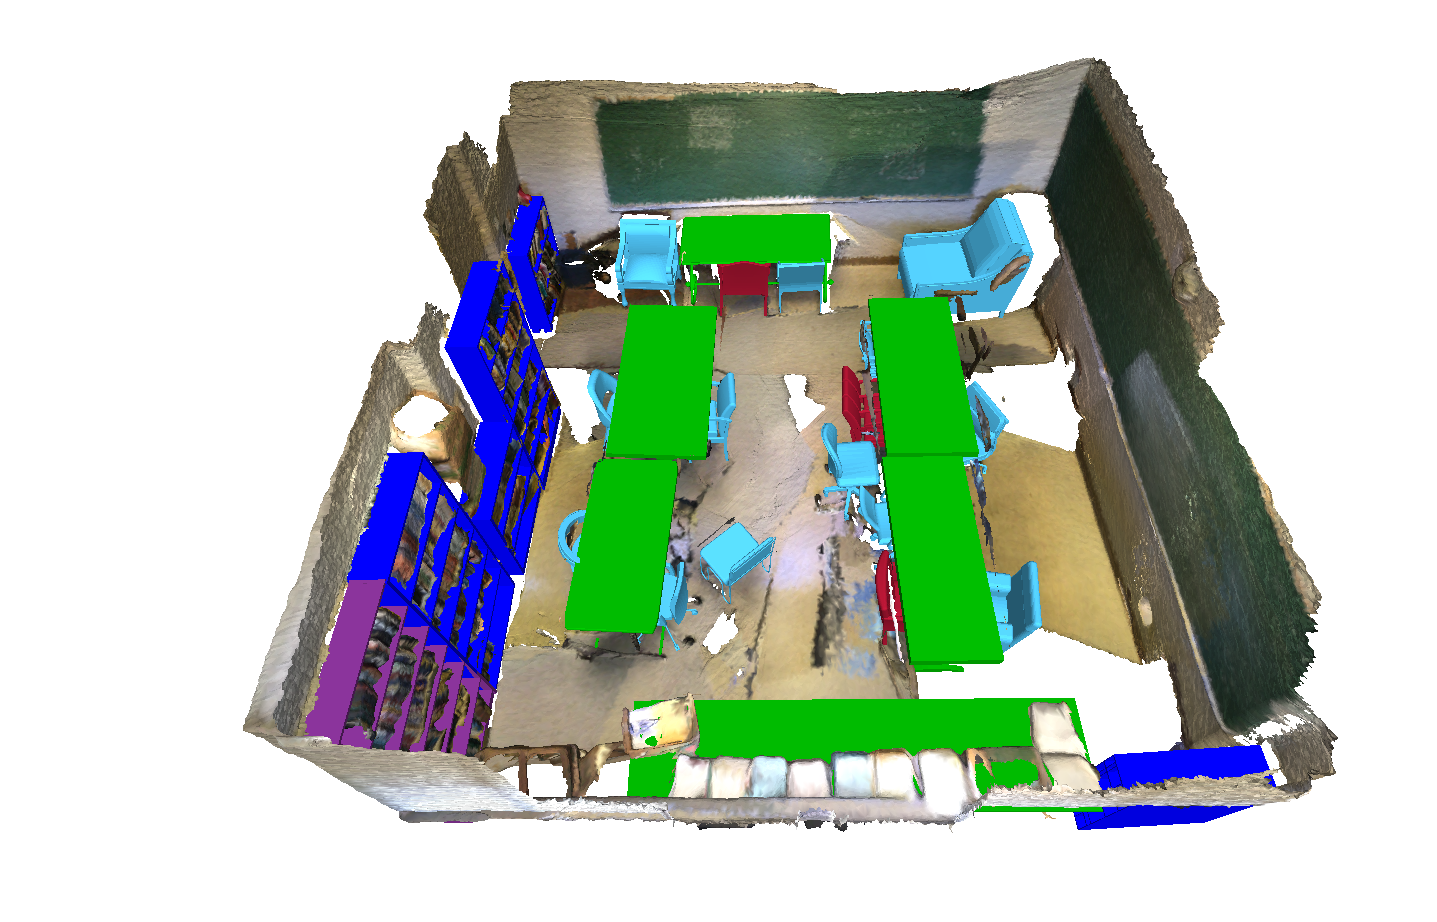} &
  \includegraphics[trim={7cm 3cm 8cm 4cm},clip,width=0.25\linewidth]{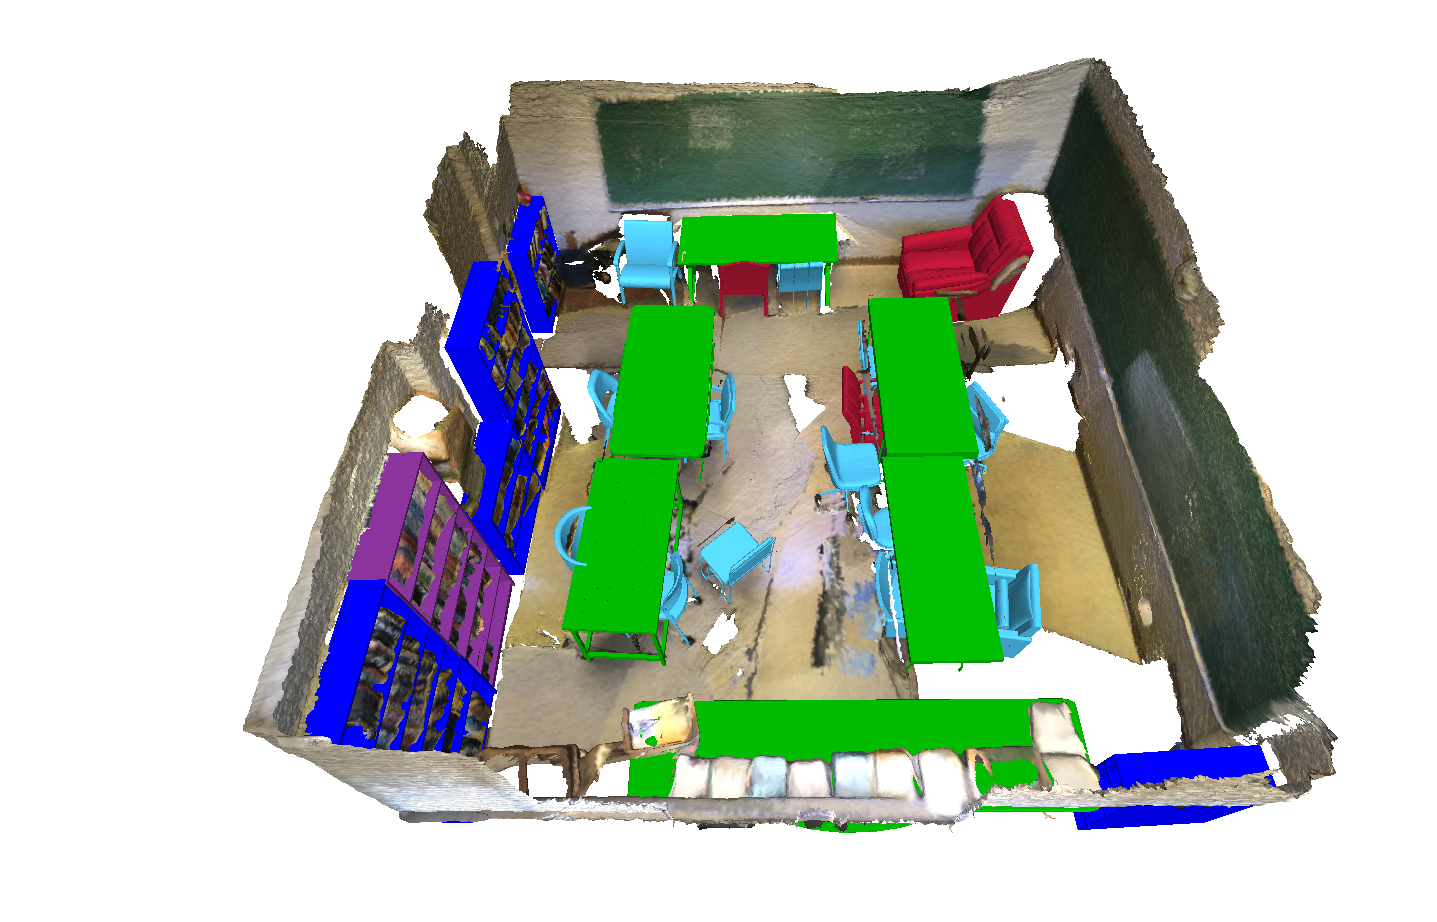} \\

     \includegraphics[trim={8cm 4cm 10cm 5cm},clip,width=0.25\linewidth]{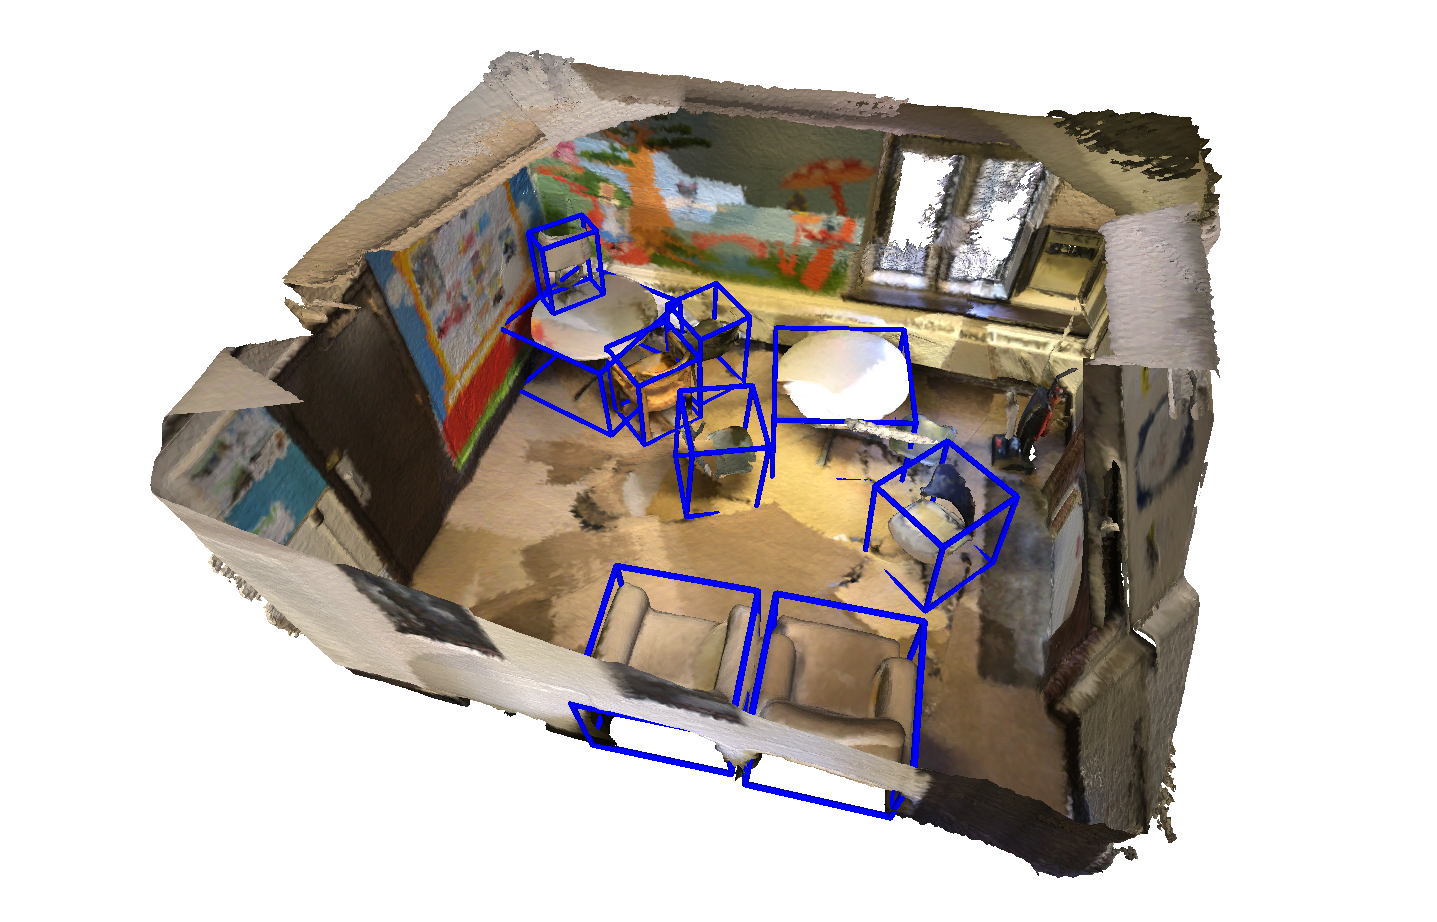} &
  \includegraphics[trim={8cm 4cm 10cm 5cm},clip,width=0.25\linewidth]{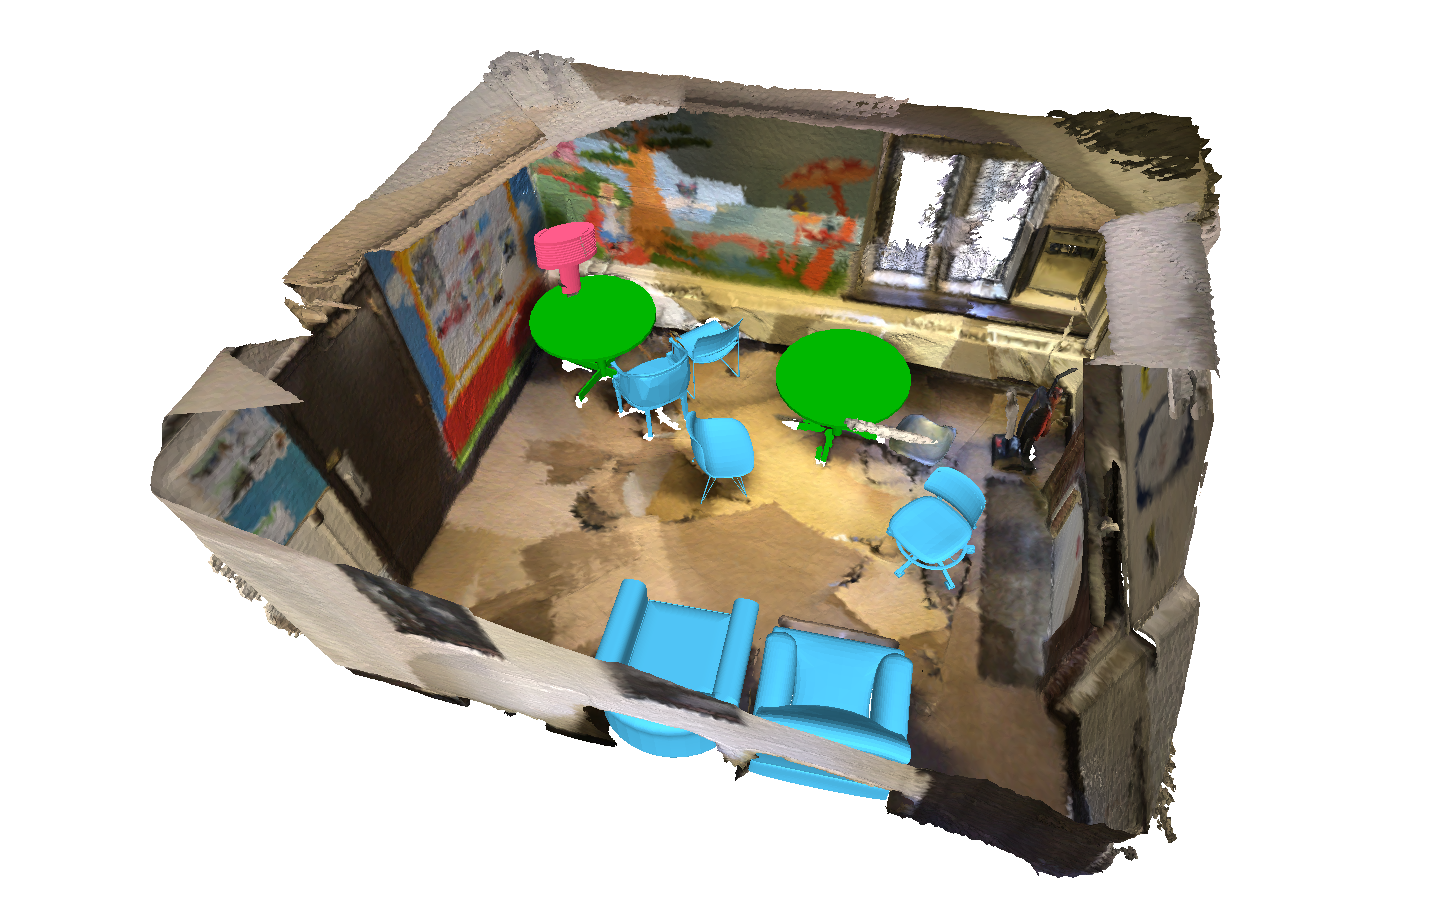} &
  \includegraphics[trim={8cm 4cm 10cm 5cm},clip,width=0.25\linewidth]{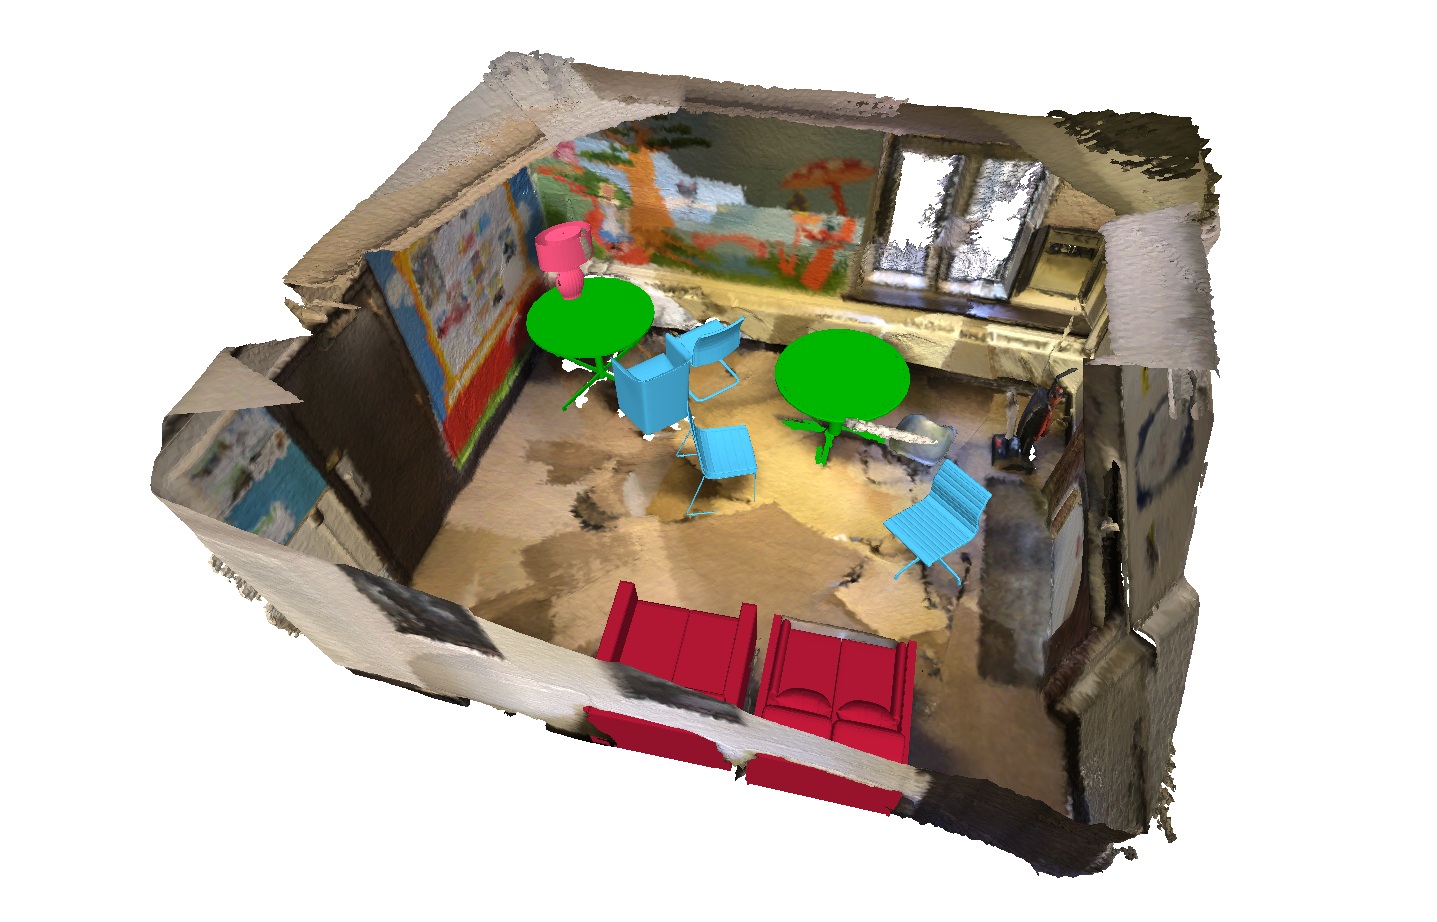} &
  \includegraphics[trim={8cm 4cm 10cm 5cm},clip,width=0.25\linewidth]{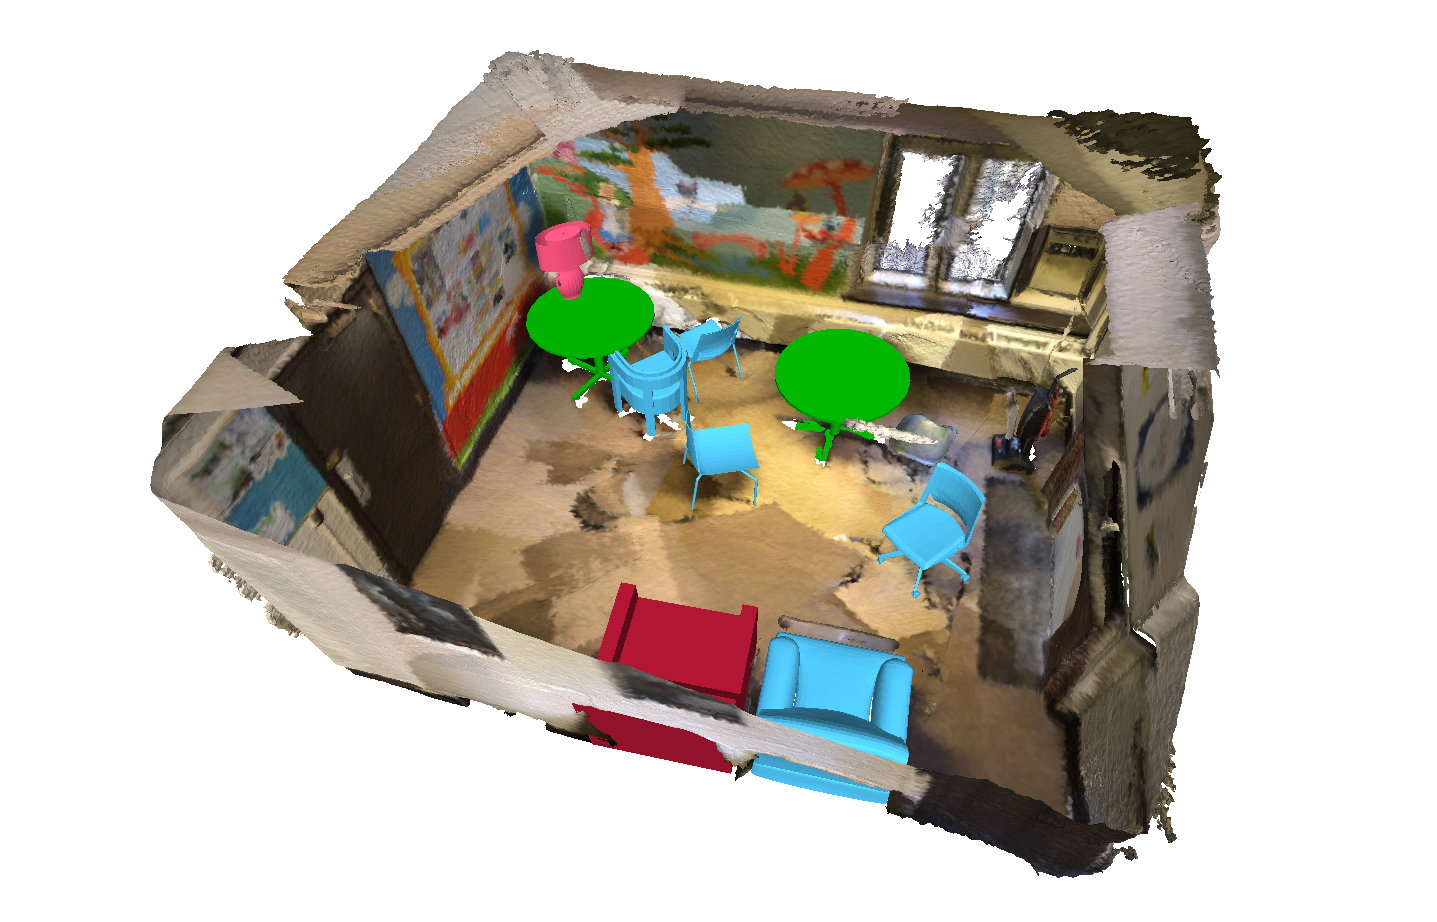} \\

  RGB-D Scan with &  Results using exh. search & HOC-Search (800 iterations)  &HOC-Search (1200 iterations) \\
   initial 3D boxes         &   \textbf{with category label}   &      without category label    & without category label\\
\end{tabular}
}
\caption{
\stefan{
Qualitative results for CAD model and pose retrieval for objects with unknown category label.
From left to right, we show 1) the input scan with initial 3D boxes, 2) the CAD models retrieved with exhaustive search \textbf{and} ground-truth category label as reference result, and 3) - 4) the results of HOC-Search for unknown category labels for 800 and 1200 iterations, respectively. Although the complexity for retrieval highly increases with unknown category labels, HOC-Search is able to find suitable CAD models and predict the correct object poses. Note that HOC-Search does not always retrieve the same category label as in the ground-truth, however, this is mainly due to ambiguities of category labels (e.g. the categories Chair and Sofa share very similar CAD models, the same applies to Bookshelf and Cabinet). The color of the retrieved objects refers to the category label: \textcolor{chair_color}{Chair}, \textcolor{cabinet_color}{Cabinet}, \textcolor{bed_color}{Bed}, \textcolor{sofa_color}{Sofa}, \textcolor{table_color}{Table}, \textcolor{bookshelf_color}{Bookshelf}, \textcolor{lamp_color}{Lamp}, \textcolor{display_color}{Display}.
}
}
\label{fig:supp_unknown_cat}
\end{figure*}
